# Supplementary material for: Multicomponent Adaptive Sampling Configuration Interaction method in openLOWDIN: positronic and quantum nuclear systems
Source: arXiv:2611.21790 source file (2026-11-16)
Supplement: Supplementary file 1 [file buffer_convergence.tex]

\section{Buffer space size convergence}
\begin{figure}[h!]
    \centering
    \includegraphics[width=0.495\linewidth]{supp_mat/Figures/hcn_buffer_sci.pdf}
    \includegraphics[width=0.495\linewidth]{supp_mat/Figures/hcn_buffer_sci+pt2.pdf}
    \includegraphics[width=0.495\linewidth]{supp_mat/Figures/hcn_buffer_scaling.pdf}
    \caption{
    Convergence of SCI energy (\textbf{a}),  SCI+PT2 energy (\textbf{b}), and total elapsed time (\textbf{c}) with respect buffer factor $b_f$, ffor a SCI calculation of HCN with 128k variational configurations. 
    }
    \label{si:fig:buffer_convergence}
\end{figure}
